# Supplementary material for: Pedagogy-R1: Pedagogically-Aligned Reasoning Model with Balanced Educational Benchmark
Source: arXiv:2505.18467 source file (2025-05-24)
Supplement: Supplementary file 1 [file 6_appendices.tex]

% \appendix
% \FloatBarrier
\newpage

% \section{Appendices}
% \label{sec:appendix}

%Table 4 
\begin{table*}[htbp!]
\small
\centering
\caption*{\raggedright \large{\textbf{Appendix 1}}}
\begin{tabular}{p{3cm}p{5cm}p{8cm}}
\toprule
\textbf{Components} & \textbf{Prompt} & \textbf{Implemented Feedback} \\ 
\midrule
\textbf{Analysis about \newline the answer} & Consider the learning history of the student and provide personalized instruction to guide the code repair and improvement.
\newline - Analyse the learners's understanding based on the problem solved by the student in the past, problem that the student just solved, and the student's answer about the problem. \newline \newline \newline \newline \newline NO PROMPTS & 
- Your solution for replacing "zap" patterns with "zp" in a given string is an intelligent utilization of string manipulation methods. The way you've implemented logic using 'for' and 'if' statements to traverse through the given string, checking for the required pattern, and substituting it, is an excellent display of skills. ... This problem requires you to utilize skills you've developed during the string manipulations exercises, but also introduces you to new concepts. (*) \newline
- The use of the for loop, string-character check, concatenation using substrings, and the if condition for 'z' and 'p' is accurate and demonstrates your capacity to grasp the problem and translating it into comprehensive logic. ... Given that you have now successfully completed problem ['492', '34'], ... (**) \newline
- I appreciate the thought process behind your solution, using a loop to go through every character in the string and then replacing every instance of "z*p" with "zp". Your usage of the substring method to achieve this replacement is clever and shows a good grasp of Java's string methods. (***)
\\ 
\textbf{Correction of \newline the answer /  \newline Tips for \newline improvement} & Utilize corrective feedback that matches the developmental stage of the learner to lead corrective feedback to learning. \newline - Never include the full version of explicit correction or improved version of the code, but provide the partial sample code that is a corrected/improved version of the current answer of the student. \newline \newline \newline \newline \newline \newline \newline NO PROMPTS & 
- While your code works well for this particular problem, there might be a potential bottleneck. You're using the 'substring' method inside a loop which could slow down the execution for large inputs dramatically because string concatenation in Java results in creation of new String object. This might not be a problem right now, but... (*) \newline
- While your solution is correct, there's a bit of optimization you could do here. Modifying a string inside a loop can be costly because it creates a new String object each time. Instead, you ought to consider using a StringBuilder, which is more efficient in memory than a String when doing many concatenations.

Here's a short sample code with StringBuilder:

```java
StringBuilder result = new StringBuilder();

for (int i = 0; i < str.length() - 2; i++) {
    // your conditions here
    result.append(str.charAt(i));  // append instead of concatenation
}

return result.toString();" (**) \newline
- Do remember though, that replacing parts of a string using this approach can be inefficient in cases where the string is very large, because strings in Java are immutable. Any modification on a string will create a new copy. So each time through the loop you are creating a new string object. You might consider using a StringBuilder in those cases... (***)
\\ 
\textbf{Positive feedback} & Give positive feedback about the student's efforts to get the answer to address students' emotions and motivation by promoting the use of emotion control and motivating strategies. \newline \newline \newline \newline \newline NO PROMPTS & 
- Good job completing the advanced string manipulation challenge! I see a lot of progress since your last session, you have come a long way from making early mistakes to now providing impressive solutions. Your hard work and dedication is evident. (*) \newline
- Great job! Your efforts have paid off and you've got the correct answer! Your progress, especially given your history with concept 492, is commendable. Stay on this path and continue the good work. (**) \newline
- Great job on solving this problem! It seems like you have a good understanding of for loops, string manipulation and control flow with if statements. Your solution is efficient and meets the problem requirements perfectly. (***)
\\ 
\textbf{Next challenge} & Provide a problem of which the difficulty is a bit higher than the one that the student just solved, only in cases where the real result that the student got for this problem is 'Correct'. & 
- As you've advanced significantly in java string manipulations and concatenations, let's move to a new area that challenges your ability to implement string-based algorithms and data structures. ... This might seem complex at first, but remember to take it one step at a time. Start by splitting the string into words, then find a way to sort them based on their length, and finally combine them back into a single string. (*) \newline
- ... I'd recommend you take a step ahead and try solving a problem that requires the use of Java's Array objects. This will further enhance your ability to manipulate and iterate over different data types effectively. The problem ['506', '37'] would be a great start! (**)
\\ 
\bottomrule
\end{tabular}
\caption{Correctness Feedback Type Generation Prompts and Implemented Feedback. The symbols *, **, and *** indicate Comparison 1, Comparison 2, and Comparison 3 respectively.}
\label{tb:correctness_feedback1}
\end{table*}

%Table 5
\begin{table*}[htbp!]
\small
\centering
\caption*{\raggedright \large{\textbf{Appendix 2}}}
\begin{tabular}{p{3cm}p{5cm}p{8cm}}
\toprule
\textbf{Components} & \textbf{Prompt} & \textbf{Implemented Feedback} \\ 
\midrule
\textbf{Related past history} & 
- You should consider the student's language and programming level when you provide feedback. \newline
- You should consider the past history of the student when you give hints. For example, you can tell the student that the student has already solved similar problems before. \newline \newline \newline NO PROMPTS
 & 
- You have already solved a similar problem earlier where you manipulated two input strings by alternating characters and appending the extra characters in case one string was longer. You even wrote a function that created n repetitions of the last n characters of a string. So, I am confident that you are capable of resolving this pattern recognition problem as well. (*) \newline
- I noticed that you successfully solved question 33 which had the same concept ID ('492') as the current problem you're working on. Remember how you overcame the challenges on that problem? Let's use that same approach here. (**) \newline
- Think about how you can create a regular expression that matches 'zap' pattern. You may need to use string concatenation or string formatting to accomplish this. (***)
\\ 
\textbf{Positive feedback} & 
Give positive feedback about the student's efforts to get the answer to address students' emotions and motivation by promoting the use of emotion control and motivating strategies. \newline \newline \newline \newline NO PROMPTS & 
- I can see you're really putting in the effort to tackle these advanced string manipulation challenges. These are complex problems and it's great to see you persevere and show determination even when the tasks are difficult. Keep going! (*) \newline
- Great job on continuously working towards understanding the concepts! I know some of these problems can be challenging, but I also know that you are determined to overcome them. Every step, even mistakes, are a learning experience! (**) \newline
- Remember, practice makes perfect. Keep solving problems like these to improve your programming skills and your understanding of string manipulation. (***)
\\ 
\textbf{Similar problems} & 
Give hints to the student like showing similar problems. \newline \newline \newline \newline \newline \newline \newline \newline NO PROMPTS & 
- You can refer to the previous problem where you manipulated the string characters to form a new string. Similarly, in this problem, you need to detect a certain pattern and replace it. Use your previous knowledge to determine how to navigate the string, recognize the pattern and make the necessary replacements. (*) \newline
- A similar problem to this is the one mentioned above (question 33). This problem required you to apply the concept '492' in a similar way. Let's revisit that problem and try to draw parallels to the current problem. (**) \newline
- This problem involves replacing part of a string with a new string. Look into Python's `str.replace(old, new)` method or you can use Python's `re.sub(pattern, repl, string)` method from the regular expression (re) module. (***)
\\ 
\textbf{Key notions \newline of the problem} & 
Give hints to the student by presenting the key notions of the problem. \newline \newline \newline \newline \newline \newline \newline \newline \newline \newline \newline \newline \newline NO PROMPTS & 
- The key concept is 'string pattern recognition'. Here, the string pattern is 'zap', where 'a' can be any character. Your task is to replace this pattern with 'zp'. Think about how you can iterate over the string and identify the pattern. Also consider string replacement methods that might help. Lastly, remember to assemble the final string in the correct order after making all necessary replacements. Keep pushing, you're making solid progress! (*) \newline
- Notice that the concept '492' requires you to understand certain key principles in programming. While tackling this problem, focus particularly on these principles and strategies that you have used before in question 33. Let's carry your previous success into this new problem. Remember, the question is not whether you will understand it but when - because with your current pace, it's only a matter of time! Keep going! (**) \newline
- Note the pattern is 'zap' where 'a' can be any character. In other words, you are looking to replace "z(any character)p" with "zp". When using regular expressions, '.' is used to represent any character and '.*' is used to represent any number of characters. (***)
\\ 
\bottomrule
\end{tabular}
\caption{Hint Feedback Type Generation Prompts and Implemented Feedback. The symbols *, **, and *** indicate Comparison 1, Comparison 2, and Comparison 3 respectively.}
\label{tb:hint_feedback2}
\end{table*}

%Table 6 
\begin{table*}[htbp!]
\small
\centering
\caption*{\raggedright \large{\textbf{Appendix 3}}}
\begin{tabular}{p{16cm}}
\toprule
\textbf{Data} \\ 
\midrule
\ A-1. The problem and correctness of each problem solved by the student in the past:\newline
\{Problem Text Past\} \newline
\newline
A-2. Problem and correctness of the problem that the student just solved: \newline
\{Problem Text Present\} \newline
\newline
A-3. The student's answer about the problem:   \newline
\{Response Code Present\}, \{Response Code AST\} \newline
\newline
A-4. The predicted probability  of the student getting this question correct:  \newline
\{Model Prob\} \newline
\newline
A-5. The real result that student got for this problem:  \newline
\{Correctness\} \newline
\newline
\newline
\newline
\ B-1. The concept IDs, question IDs, and correctness of each problem solved by the student in the past: \newline
\{Problem Past\} \newline
\newline
B-2. The concept IDs and question IDs that the student is solving: Problem and correctness of the problem that the student just solved: \newline
\{Problem Present\} \newline
\newline
B-3. The student answer about the problem:    \newline
\{Response Code Present\}, \{Response Code AST\} \newline
\newline
B-4. The predicted probability  of the student getting this question correct:   \newline
\{Model Prob\} \newline
\newline
B-5. The real result that student got for this problem: \newline
\{Correctness\} \newline
\newline
\\ 
\bottomrule
\end{tabular}
\caption{Correctness Feedback and Hint Feedback Type Generation Data.}
\label{tb:hint_feedback3}
\end{table*}

%Table 7 제목 수정 필요
\begin{table*}[htbp!]
\small
\centering
\caption*{\raggedright \large{\textbf{Appendix 4}}}
\begin{tabular}{p{2cm}p{6.5cm}p{6.5cm}}
\toprule
\textbf{Case} & \textbf{Prompt} & \textbf{Student Answer} \\ 
\midrule
\textbf{Comparison 1} & 
\#\#\# Situation \& Role \newline
You are a teacher who evaluates a student's programming skills and provides feedback. The below outlines the part of learning history of the student you are tutoring and guidelines that you should consider as a teacher, conducting a one-on-one lesson. 
\newline \newline
\#\#\# Guidelines for the Teacher \newline
1. Consider the learning history of the student and provide personalized instruction to guide the code repair and improvement. \newline
- Analyse the learners's understanding based on the problem solved by the student in the past, a problem that the student just solved, and the student's answer about the problem. \newline
2. Utilize corrective feedback which matches with the developmental stage of the learner, in order to lead corrective feedback to learning. \newline
- Provide analysis about the answer code of the student with explicit code that the student submitted. \newline
- Never include the full version of explicit correction or improved version of the code, but provide the partial sample code that is a corrected/improved version of the current answer of the student. \newline
3. Give positive feedback about the student's efforts to get the answer to address students' emotions and motivation by promoting the use of emotion control and motivating strategies. \newline
4. Provide a problem of which the difficulty is a bit higher than the ""Problem that the student just solved"" only in cases of '5. The real result that student got for this problem' is 'Correct'. \newline
\newline
\#\#\# Learning history \newline
1. The problem and correctness of each problem solved by the student in the past:\newline
\{Problem Text Past\} \newline
\newline
2. Problem that the student just solved: \newline
\{Problem Text Present\} \newline
\newline
3. The student's answer about the problem: \newline
\{Response Code Present\}, \{Response Code AST\} \newline
\newline
4. The predicted probability  of the student getting this question correct: \newline
\{Model Prob\} \newline
\newline
5. The real result that student got for this problem: \newline
\{Correctness\} \newline
\newline
\#\#\# Output form: \newline
1. Positive feedback \newline
2. Analysis about the answer \newline
3. Correction of the answer / Tips for improvement \newline
4. Next challenge (provide this only in cases of '5. The real result that student got for this problem' is 'Correct')
comments for cheering up \newline
\newline
\#\#\# Instruction \newline
Refer to the past history, predicted probability of the student getting this question correct, and the real result that the student got for this problem, Provide appropriate feedback to the student in that situation. 
 & 
1. Positive feedback: \newline
   Good job completing the advanced string manipulation challenge! I see a lot of progress since your last session, you have come a long way from making early mistakes to now providing impressive solutions. Your hard work and dedication is evident. \newline
\newline
2. Analysis about the answer: \newline
   Your solution for replacing ""zap"" patterns with ""zp"" in a given string is an intelligent utilization of string manipulation methods. The way you've implemented logic using 'for' and 'if' statements to traverse through the given string, checking for the required pattern, and substituting it, is an excellent display of skills. You are proficiently laying out your control structures and syntax very well. \newline
\newline
3. Correction of the answer / Tips for improvement: \newline
   While your code works well for this particular problem, there might be a potential bottleneck. You're using the 'substring' method inside a loop which could slow down the execution for large inputs dramatically because string concatenation in Java results in creation of new String object. This might not be a problem right now, but it's beneficial to keep in mind the performance aspect while programming. As an improvement try using 'StringBuilder' or 'StringBuffer' implementations which can handle such operations more efficiently. \newline
\newline
4. Next challenge:
\newline
   As you've advanced significantly in java string manipulations and concatenations, let's move to a new area that challenges your ability to implement string-based algorithms and data structures. 
\newline \newline
   Here's a problem for you to solve:
   \newline
   Write a function that takes a string as input, which consists of words separated by spaces, and returns a new string where the words are sorted in the order of their length. If multiple words have the same length, they should retain their original order.
   \newline
   This might seem complex at first, but remember to take it one step at a time. Start by splitting the string into words, then find a way to sort them based on their length, and finally combine them back into a single string. This problem requires you to utilize skills you've developed during the string manipulations exercises, but also introduces you to new concepts. Good luck!
\\ 
\\ 
\bottomrule
\end{tabular}
\caption{Comparison 1: Prompts and Student Answer in Correctness Feedback Type}
\label{tb:hint_feedback4}
\end{table*}

%Table 8 제목 수정 필요
\begin{table*}[htbp!]
\small
\centering
\caption*{\raggedright \large{\textbf{Appendix 5}}}
\begin{tabular}{p{2cm}p{6.5cm}p{6.5cm}}
\toprule
\textbf{Case} & \textbf{Prompt} & \textbf{Student Answer} \\ 
\midrule
\textbf{Comparison 2} & 
\#\#\# Situation \& Role \newline
You are a teacher who evaluates a student's programming skills and provides feedback. The below outlines the part of learning history of the student you are tutoring and guidelines that you should consider as a teacher, conducting a one-on-one lesson. 
\newline \newline
\#\#\# Guidelines for the Teacher \newline
1. Consider the learning history of the student and provide personalized instruction to guide the code repair and improvement. \newline
- Analyse the learners's understanding based on the problem solved by the student in the past, the problem that the student just solved, and the student's answer about the problem. \newline
2. Utilize corrective feedback which matches with the developmental stage of the learner, in order to lead corrective feedback to learning. \newline
- Provide analysis about the answer code of the student with explicit code that the student submitted. \newline
- Never include the full version of explicit correction or improved version of the code, but provide the partial sample code that is a corrected/improved version of the current answer of the student. \newline
3. Give positive feedback about the student's efforts to get the answer to address students' emotions and motivation by promoting the use of emotion control and motivating strategies. \newline
4. Provide a problem of which the difficulty is a bit higher than the ""Problem that the student just solved"" only in cases of '5. The real result that student got for this problem' is 'Correct'. \newline
\newline
\#\#\# Learning history \newline
1. The concept IDs, question IDs, and correctness of each problem solved by the student in the past:\newline
\{Problem Past\} \newline
\newline
2. The concept IDs and question IDs that the student is solving: \newline
\{Problem Present\} \newline
\newline
3. The student answer about the problem:  \newline
\{Response Code Present\}, \{Response Code AST\} \newline
\newline
4. The predicted probability  of the student getting this question correct: \newline
\{Model Prob\} \newline
\newline
5. The real result that student got for this problem:  \newline
\{Correctness\} \newline
\newline
\#\#\# Output form: \newline
1. Positive feedback \newline
2. Analysis about the answer \newline
3. Correction of the answer / Tips for improvement \newline
4. Next challenge (provide this only in cases of '5. The real result that student got for this problem' is 'Correct')
comments for cheering up \newline
\newline
\#\#\# Instruction \newline
Refer to the past history, predicted probability of the student getting this question correct, and the real result that the student got for this problem, Provide appropriate feedback to the student in that situation. 
 & 
1. Positive feedback: \newline
Great job! Your efforts have paid off and you've got the correct answer! Your progress, especially given your history with concept 492, is commendable. Stay on this path and continue the good work. 
 \newline
\newline
2. Analysis about the answer: \newline
Your interpretation of the problem and implementation of the solution display a good grasp of Java's string manipulation mechanisms and condition-based programming. The use of the for loop, string-character check, concatenation using substrings, and the if condition for 'z' and 'p' is accurate and demonstrates your capacity of grasping the problem and translating it into comprehensive logic.\newline
\newline
3. Correction of the answer / Tips for improvement: \newline
While your solution is correct, there's a bit of optimization you could do here. Modifying a string inside a loop can be costly because it creates a new String object each time. Instead, you ought to consider using a StringBuilder, which is more efficient in memory than a String when doing many concatenations. Note that this does not affect the correctness of your solution; it is just a suggestion to improve the performance.

Here's a short sample code with StringBuilder:

```java
StringBuilder result = new StringBuilder();

for (int i = 0; i < str.length() - 2; i++) {
    // your conditions here
    result.append(str.charAt(i));  // append instead of concatenation
}

return result.toString();
``` \newline
\newline
4. Next challenge:
\newline
Only provide this in cases of '5. The real result that student got for this problem' is 'Correct'. Given that you have now successfully completed problem ['492', '34'], I'd recommend you take a step ahead and try solving a problem that requires the use of Java's Array objects. This will further enhance your ability to manipulate and iterate over different data types effectively. The problem ['506', '37'] would be a great start! Keep pushing yourself!
\\ 
\\ 
\bottomrule
\end{tabular}
\caption{Comparison 2: Prompts and Student Answer in Correctness Feedback Type}
\label{tb:hint_feedback5}
\end{table*}

%Table 9 제목 수정 필요
\begin{table*}[htbp!]
\small
\centering
\caption*{\raggedright \large{\textbf{Appendix 6}}}
\begin{tabular}{p{2cm}p{6.5cm}p{6.5cm}}
\toprule
\textbf{Case} & \textbf{Prompt} & \textbf{Student Answer} \\ 
\midrule
\textbf{Comparison 3} & 
\#\#\# Situation \& Role \newline
You are a teacher who evaluates a student's programming skills and provides feedback.
\newline \newline
\#\#\# Learning history \newline
1. The problem and correctness of each problem solved by the student in the past:\newline
\{Problem Text Past\} \newline
\newline
2. Problem that the student just solved: \newline
\{Problem Text Present\} \newline
\newline
3. The student answer about the problem:  \newline
\{Response Code Present\}, \{Response Code AST\} \newline
\newline
4. The predicted probability  of the student getting this question correct: \newline
\{Model Prob\} \newline
\newline
5. The real result that student got for this problem:  \newline
\{Correctness\} \newline
\newline
\#\#\# Instruction \newline
Provide appropriate feedback to the student in that situation.
 & 
Great job on solving this problem! It seems like you have a good understanding of for loops, string manipulation and control flow with if statements. Your solution is efficient and meets the problem requirements perfectly. 
 \newline
\newline
I appreciate the thought process behind your solution, using a loop to go through every character in the string and then replacing every instance of "z*p" with "zp". Your usage of the substring method to achieve this replacement is clever and shows a good grasp of Java's string methods.\newline
\newline
Do remember though, that replacing parts of a string using this approach can be inefficient in cases where the string is very large, because strings in Java are immutable. Any modification on a string will create a new copy. So each time through the loop you are creating a new string object. \newline
\newline
You might consider using a StringBuilder in those cases, which is mutable and allows modifications to the string it holds without creating new string objects. However, for a function of this size, your solution is fine. \newline
\newline
Keep up the good work!
\\ 
\\ 
\bottomrule
\end{tabular}
\caption{Comparison 3: Prompts and Student Answer in Correctness Feedback Type}
\label{tb:hint_feedback6}
\end{table*}

%Table 10 제목 수정 필요
\begin{table*}[htbp!]
\small
\centering
\caption*{\raggedright \large{\textbf{Appendix 7}}}
\begin{tabular}{p{2cm}p{6.5cm}p{6.5cm}}
\toprule
\textbf{Case} & \textbf{Prompt} & \textbf{Student Answer} \\ 
\midrule
\textbf{Comparison 1} & 
\#\#\# Situation \& Role \newline
You are a teacher who evaluates a student's programming skills and provides feedback. The below outlines the part of learning history of the student you are tutoring and guidelines that you should consider as a teacher, conducting a one-on-one lesson.  
\newline \newline
\#\#\# Guidelines for feedback \newline
1. You should consider the student's language and programming level when you provide feedback. \newline
2. Give positive feedback about the student's efforts to get the answer to address students' emotions and motivation by promoting the use of emotion control and motivating strategies. \newline
3. Give hints to the student like showing similar problems and presenting the key notions of the problem. \newline
4. You should consider the past history of the student when you give hints. For example, you can tell the student that the student has already solved similar problems before. \newline
\newline
\#\#\# Learning history \newline
1. The problem and correctness of each problem solved by the student in the past:\newline
\{Problem Text Past\} \newline
\newline
2. Problem that the student just solved: \newline
\{Problem Text Present\} \newline
\newline
3. The predicted probability  of the student getting this question correct: \newline
\{Model Prob\} \newline
\newline
\newline
\#\#\# Output form: \newline
1. Positive feedback \newline
2. Related past history \newline
3. Similar problems \newline
4. Key notions of the problem
\newline
\newline
\#\#\# Instruction \newline
Refer to the past history, past problems that the student solved, and predicted probability of the student getting this question correct for this problem. Provide appropriate hints to the student in that situation.
 & 
1. Positive feedback \newline
I can see you're really putting in the effort to tackle these advanced string manipulation challenges. These are complex problems and it's great to see you persevere and show determination even when the tasks are difficult. Keep going!
 \newline
\newline
2. Related past history \newline
You have already solved a similar problem earlier where you manipulated two input strings by alternating characters and appending the extra characters in case one string was longer. You even wrote a function that created n repetitions of the last n characters of a string. So, I am confident that you are capable of resolving this pattern recognition problem as well.\newline
\newline
3. Similar problems \newline
You can refer to the previous problem where you manipulated the string characters to form a new string. Similarly, in this problem, you need to detect a certain pattern and replace it. Use your previous knowledge to determine how to navigate the string, recognize the pattern, and make the necessary replacements.\newline
\newline
4. Key notions of the problem
\newline
The key concept is 'string pattern recognition'. Here, the string pattern is 'zap', where 'a' can be any character. Your task is to replace this pattern with 'zp'. Think about how you can iterate over the string and identify the pattern. Also consider string replacement methods that might help. Lastly, remember to assemble the final string in the correct order after making all necessary replacements. Keep pushing, you're making solid progress!
\\ 
\\ 
\bottomrule
\end{tabular}
\caption{Comparison 1: Prompts and Student Answer in Hint Feedback Type}
\label{tb:hint_feedback7}
\end{table*}

%Table 11 제목 수정 필요
\begin{table*}[htbp!]
\small
\centering
\caption*{\raggedright \large{\textbf{Appendix 8}}}
\begin{tabular}{p{2cm}p{6.5cm}p{6.5cm}}
\toprule
\textbf{Case} & \textbf{Prompt} & \textbf{Student Answer} \\ 
\midrule
\textbf{Comparison 2} & 
\#\#\# Situation \& Role \newline
You are a teacher who evaluates a student's programming skills and provides feedback. The below outlines the part of learning history of the student you are tutoring and guidelines that you should consider as a teacher, conducting a one-on-one lesson.  
\newline \newline
\#\#\# Guidelines for feedback \newline
1. You should consider the student's language and programming level when you provide feedback. \newline
2. Give positive feedback about the student's efforts to get the answer to address students' emotions and motivation by promoting the use of emotion control and motivating strategies. \newline
3. Give hints to the student like showing similar problems and presenting the key notions of the problem. \newline
4. You should consider the past history of the student when you give hints. For example, you can tell the student that the student has already solved similar problems before. \newline
\newline
\#\#\# Learning history \newline
1. The concept IDs, question IDs, and correctness of each problem solved by the student in the past:\newline
\{Problem Past\} \newline
\newline
2. The concept IDs and question IDs that the student is solving:\newline
\{Problem Present\} \newline
\newline
3. The predicted probability  of the student getting this question correct:  \newline
\{Model Prob\} \newline
\newline
\newline
\#\#\# Output form: \newline
1. Positive feedback \newline
2. Related past history \newline
3. Similar problems \newline
4. Key notions of the problem
\newline
\newline
\#\#\# Instruction \newline
Refer the past history, past problems that the student solved, predicted probability of the student getting this question correct for this problem. Provide appropriate hints to the student in that situation.
 & 
1. Positive feedback \newline
Great job on continuously working towards understanding the concepts! I know some of these problems can be challenging, but I also know that you are determined to overcome them. Every step, even mistakes, are a learning experience!
 \newline
\newline
2. Related past history \newline
I noticed that you successfully solved question 33 which had the same concept ID ('492') as the current problem you're working on. Remember how you overcame the challenges on that problem? Let's use that same approach here.\newline
\newline
3. Similar problems \newline
A similar problem to this is the one mentioned above (question 33). This problem required you to apply the concept '492' in a similar way. Let's revisit that problem and try to draw parallels to the current problem.\newline
\newline
4. Key notions of the problem
\newline
Notice that the concept '492' requires you to understand certain key principles in programming. While tackling this problem, focus particularly on these principles and strategies that you have used before in question 33. Let's carry your previous success into this new problem. Remember, the question is not whether you will understand it but when - because with your current pace, it's only a matter of time! Keep going!
\\ 
\\ 
\bottomrule
\end{tabular}
\caption{Comparison 2: Prompts and Student Answer in Hint Feedback Type}
\label{tb:hint_feedback8}
\end{table*}

%Table 12 제목 수정 필요
\begin{table*}[htbp!]
\small
\centering
\caption*{\raggedright \large{\textbf{Appendix 9}}}
\begin{tabular}{p{2cm}p{6.5cm}p{6.5cm}}
\toprule
\textbf{Case} & \textbf{Prompt} & \textbf{Student Answer} \\ 
\midrule
\textbf{Comparison 3} & 
\#\#\# Situation \& Role \newline
You are a teacher who evaluates a student's programming skills and provides feedback.  
\newline \newline
\#\#\# Learning history \newline
1. The problem and correctness of each problem solved by the student in the past:\newline
\{Problem Text Past\} \newline
\newline
2. Problem that the student just solved:\newline
\{Problem Text Present\} \newline
\newline
3. The predicted probability  of the student getting this question correct: \newline
\{Model Prob\} \newline
\newline
\newline
\#\#\# Instruction \newline
Provide appropriate hints to the student in that situation.
 & 
To solve this problem, you need to focus on string manipulation methods. Here are some hints to consider: \newline
\newline
1. This problem involves replacing part of a string with a new string. Look into Python's `str.replace(old, new)` method or you can use Python's `re.sub(pattern, repl, string)` method from the regular expression (re) module.
 \newline
\newline
2. Note the pattern is 'zap' where 'a' can be any character. In other words, you are looking to replace ""z(any character)p"" with ""zp"". When using regular expressions, '.' is used to represent any character and '.*' is used to represent any number of characters.\newline
\newline
3. Think about how you can create a regular expression that matches 'zap' pattern. You may need to use string concatenation or string formatting to accomplish this.
\newline
\newline
4. Write down the steps of the problem and try to follow them while creating your solution. It is a good practice to first solve it manually for a given string and then code it for the generalized problem. 
\newline
\newline
Remember, practice makes perfect. Keep solving problems like these to improve your programming skills and your understanding of string manipulation.
\\ 
\\ 
\bottomrule
\end{tabular}
\caption{Comparison 3: Prompts and Student Answer in Hint Feedback Type}
\label{tb:hint_feedback9}
\end{table*}
